# Supplementary material for: Constrained Conditional Moment Restriction Models
Source: arXiv:1509.06311 source file (2022-04-28)
Supplement: Supplementary file 1 [file AppExamplesProofs.tex]

\section{Illustrative Examples} \label{sec:examplesproofs}

We next examine special cases of our general analysis and illustrate both how to implement our procedure and verify the assumptions in the main text.

\input{Appendix/ExGMMProofs} % Example: GMM

\input{Appendix/ExNPIVProofs}     % Example: NPIV with Slutsky

\input{Appendix/ExQuantProofs}    % Example: Quantile

\input{Appendix/ExDemandProofs}   % Example: Demand 
